# Supplementary material for: Statistical and Thermodynamical Studies of the Strongly Interacting Matter
Source: arXiv:1605.08619 ancillary file (2016-07-26)
Supplement: Supplementary file 1 [file questions_from_reviewers.pdf]

# Questions from the reviewers

## Question 1

What are the physical motivations for the specific examples of the energy-addition rules used in Chapter II.?

## Answer

The addition rules we used in our investigations are summarized in Table 1. In both cases the "strength" of the modification is set up such a way that the modified sum for two particles with average kinetic energy is proportional to the same value:  $\langle E \rangle \oplus \langle E \rangle = \langle E \rangle + \langle E \rangle + \frac{a}{\langle E \rangle} \langle E \rangle^2 = (2 + a) \langle E \rangle$ . A composition rule like this leads to scaling solutions in the two component case, when the modification parameter  $a^{AB}$  is different from  $a^{AA}$  and  $a^{BB}$  ( $A$  and  $B$  denote the two species of particles).

In our numerical simulations, case I. means constant and different  $a$  parameters for each particle species, whilst in case II.  $a^{AB}$  is different from  $a^{AA}$  and  $a^{BB}$  only above an energy scale  $\Lambda_0 \langle E \rangle$ . Therefore, the system behaves effectively as a one-component gas for certain regions of the phase space. These two examples are not *primarily* motivated physically. The question rather was how we can change the time-dependence of the average kinetic energy. For positive modification parameters in case II. this can result in solutions with either the growing or lowering of  $\langle E \rangle$ , depending on the value of  $\Lambda_0$ .

|                        | I.) ( $a_0, a_1$ )                 | II.) ( $a_0, a_1, \Lambda_0$ )                                                                                                                                               |
|------------------------|------------------------------------|------------------------------------------------------------------------------------------------------------------------------------------------------------------------------|
| $A^{AA} = A^{BB}$      | $\frac{a_0}{\langle E \rangle}$    | $\frac{a_0}{\langle E \rangle}$                                                                                                                                              |
| $A^{AB} = A^{BA}$      | $\frac{a_1}{\langle E \rangle}$    | $\frac{a_0}{\langle E \rangle}, \text{ if } E_1 + E_2 < \Lambda_0 \langle E \rangle$<br>$\frac{a_1}{\langle E \rangle}, \text{ if } E_1 + E_2 > \Lambda_0 \langle E \rangle$ |
| long time<br>behaviour | increase of<br>$\langle E \rangle$ | increase or decrease of<br>$\langle E \rangle$                                                                                                                               |

Table 1: The two cases we investigated numerically, with modification parameters scaled down by  $\langle E \rangle$ .  $a_0$ ,  $a_1$  and  $\Lambda_0$  are positive constants.

## Question 2

Is it not problematic to describe "thermalization" using a model which is not in thermal equilibrium, however, the expression for the modification of the kinetic energy addition remains the same during the whole time-evolution?

## Answer

Our two-component toy model reaches a stationary state only if the modification parameters in the kinetic energy addition rule change with time. This can occur by the dynamical feedback of the type  $a(\langle E \rangle) \sim 1/\langle E \rangle$ , for example. The relaxation time to this stationary state depends on the details of the feedback mechanism.

It is worth mentioning that despite the lack of a detailed balance solution, the system is in a "prethermalized" state: This means that the equation of state – for example the relation  $S(\langle E \rangle)$  for the Boltzmann entropy – is already stabilized.

### Question 3

The assumption that the source pairs are aligned in parallel to each other is rather unrealistic. In what extent does the distribution of the pair directions weaken the effect?

### Answer

One can assume a random distortion compared to the direction  $\varphi = 0$ . The calculation discussed in Eq. (3.13) of Section 3.5 is to be redone:

$$\bar{Y} = \int_{\delta_{\min}}^{\delta_{\max}} d\delta g(\delta) \int_0^{2\pi} d\tilde{\varphi} Y_0 (1 + 2v_2 \cos[2(2\tilde{\varphi} - \varphi + \delta)]) \frac{r^2(\tilde{\varphi})}{2} = \quad (1)$$

$$= Y_0 T + 2Y_0 T \underbrace{F v_2}_{=\bar{v}_2} \int_{\delta_{\min}}^{\delta_{\max}} d\delta g(\delta) \cos(2\varphi - 2\delta) = \quad (2)$$

$$= Y_0 T \left( 1 + 2\bar{v}_2 \cos(2\varphi) \int_{\delta_{\min}}^{\delta_{\max}} d\delta g(\delta) \cos(2\delta) \right) =: Y_0 T (1 + 2C \cdot \bar{v}_2 \cos(2\varphi)). \quad (3)$$

In case of a Gaussian-like distribution:  $g(\delta) \sim e^{-\frac{\delta^2}{2\Delta^2}}$  – which is properly restricted in  $\delta$  to the interval  $[-\pi, \pi]$  – we get the suppression factor  $C \sim e^{-2\Delta^2}$ . Assuming that  $\Delta$  is determined only by the initial state of the collision (e.g. by the average energy density)  $C$  can be absorbed into the geometric form factor  $F$  discussed in Section 3.5.

It would be most interesting to estimate the magnitude of  $\Delta$ . This, however, cannot be done without modeling the mechanism which orders the source pairs. At this point, unfortunately, we do not know anything quantitative about such a potential mechanism.

### Question 4

At the end of Section 3.6 it is mentioned that it would be interesting to investigate higher flow coefficients such as  $v_3, v_4$  etc. Why is that a problem, since expressions similar to Eq. (3.11) can be deduced for all the even  $v_n$ <sup>1</sup>.

### Answer

We emphasized in Section 3.6 that *radiation sources with symmetry other than the dipole-like* might exist, and those may contribute to the higher flow harmonics considerably. For the source-pair, the (phase-shift averaged) coefficients  $v_{2n}$  for  $n > 1$  can be derived similarly to Eq. (3.11), but one has to substitute  $J_2$  with  $(-1)^n J_{2n}$  in the nominator of the formula. For example, the corresponding  $\langle v_4 \rangle$  starts with negative values – see Fig. 1 –, which clearly contradicts the experimental findings.

It would be worth investigating though, how radiating objects with higher asymmetry can contribute to the higher flow coefficients, see for example [1] for a particular approach. Our model, however, needs to be generalized to tackle such questions.

---

<sup>1</sup> $\langle v_n \rangle$  equals zero for odd  $n$  after the phase-shift averaging.

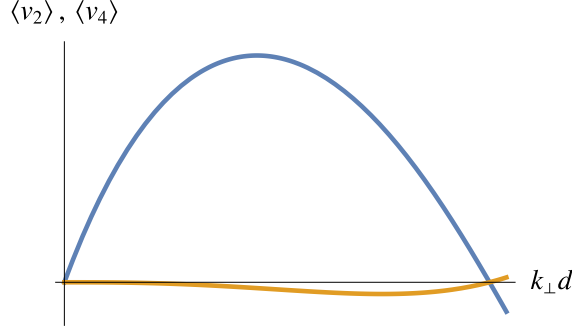

Figure 1: Phase-shift averaged flow harmonics  $\langle v_2 \rangle$  (blue) and  $\langle v_4 \rangle$  (orange) as a function of the transverse momentum  $k_\perp$  of the emitted particles times the distance  $d$  of the two sources. Curves are derived using the same source-pair ensemble.

### Question 5

How is the expression of the fluidity measure  $\eta/s$  in Eq. (4.35) compatible with  $\eta/s$  in Eq. (4.31). The latter has the lower bound  $1/\pi$ , while the former obviously does not have such a bound.

### Answer

The main difference is that for Eq. (4.31) the microcausal Lorentz-ansatz of Eq. (4.28) was used, whilst for Eq. (4.35) we mimicked the "real particle" behavior by putting Dirac-delta into Eqs. (4.6-4.7). In these latter formulas the microcausality is artificially built-in, therefore this is not the small- $\gamma$  limit of Eq. (4.28), although both calculation result the  $\eta/s \sim \gamma^{-1}$  behavior<sup>2</sup>.

We note that  $\eta/s$  approaching zero does not contradict the lower bound  $\sim s/T^3$  which follows from the extended quasi-particle model. In case of the Dirac-delta spectral function this inequality gives an *upper* bound for the value of  $\gamma$ , which turns out to be proportional to the temperature  $T$ :

$$\frac{T^2}{\gamma m} \geq \frac{s}{IT^3} = \frac{1}{2\pi^2 I} \frac{m^3}{T^3} K_3(m/T),$$

$$\underbrace{\frac{T}{\frac{1}{2\pi^2 I} \max_y \{y^4 K_3(y)\}}}_{\approx 89.98 \cdot T} \geq \gamma.$$

### Question 6

What does justify the approximation made in Eq. (4.38): namely, neglecting all contribution but  $p = M$  in the integrals? According to Fig. 4.5, the spectral function has a wide continuum part. Why does that not count?

### Answer

The integrand  $g(p)$  in question is proportional *not only* to the spectral function but to  $\frac{\partial K}{\partial p}$  as well. In this case,  $K$  behaves step-like near  $p = M$ , so  $g(p)$  approximates a Dirac-delta better and better as the step becomes steeper. Therefore the integrand in  $p = M$  gives an increasingly accurate value for the integral as  $\epsilon \rightarrow 0$ .

<sup>2</sup>The temperature dependence is, however, different.

## Question 7

How one could improve the mean-field critical exponents mentioned in Chapter 4? What about the correlation functions for that matter?

## Answer

To exceed the Gaussian type generating functional, one need to take into account higher terms in  $\varphi$  despite the nonlocal quadratic one – i.e. turning on the interaction. With interaction terms, Wick's theorem would not connect all the correlation functions like it does in the EQP framework. It is safe to say, that most of the nonperturbative methods used to deal with interacting QFTs can be generalized using a nonlocal quadratic term instead of the local one. For example, in the case of the so-called 2PI resummation, the starting point of the method is a nonlocal quadratic term, which is to be determined self-consistently.

Taking the  $\varphi^2$ -term given, also Feynman's rules can be worked out in the usual way. The main difference is that the propagator-lines now represent the retarded propagator corresponding to  $K$ , i.e.:  $\int_p \frac{\rho(q)}{p-q+i0^+}$ . Renormalization of the tree-level vertices would be needed, but this can be done by using local counter-terms – at least when the large- $p$  asymptotic of  $K^{-1}$  is the same as that of the free propagator.

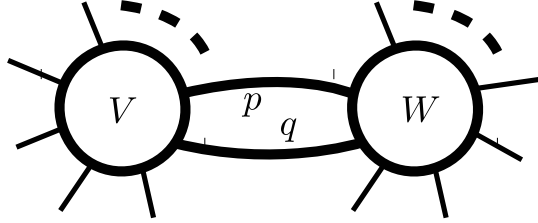

Figure 2: A sketch of a one-loop correction to vertices.  $V$  and  $W$  represent vertex functions, the propagator lines are the ones corresponding to  $K^{-1}$ .

There is an illustrative example of a "one-loop correction" depicted on Fig. 2. The vertex functions  $V(p, q, \dots)$  and  $W(p, q, \dots)$  are connected through two propagator lines. This gives the following contribution:

$$\sim \int_r \rho(r) \int_s \rho(s) \int_p \int_q \frac{i}{p-r+i0^+} \frac{i}{q-s+i0^+} V(p, q, \dots) W(p, q, \dots). \quad (4)$$

To put it simply, one has to integrate all the usual diagrams weighted by the spectral function  $\rho$ .

Introducing such interaction terms raises the question though: Is the above-mentioned perturbative expansion – done on the level of the effective theory – somehow in connection with the perturbation theory defined on the level of the fundamental theory, as a resummation of certain class of graphs, for example?

## Question 8

Are there data accessible concerning the spectral functions of certain quantum channels? If so, can one use that to describe the thermodynamical properties of the given material?

## Answer

There are indeed measured data from which one can deduce the spectral functions of certain quantum channels of the strongly interacting matter. These data are usually from electron-positron experiments, like the ALEPH [2] and OPAL [3] which were run in CERN's LEP program. The subject of these experiments were the decay products of quark pairs induced by high-energy lepton pairs. The medium-modification of hadronic spectral functions<sup>3</sup> was investigated in the CERN SPS NA60 [4] experiment by colliding protons.

Depending on the quantum numbers of the identified particles, the spectral function of  $\langle q\bar{q} \rangle$  can be probed with some assumptions. The optical theorem relates the measured decay rates with the self-energy contribution of the interaction which controls the decay in question<sup>4</sup>. Now supposing that data concerning all the relevant decay channels are known, the self-energy – and the spectral function, consequently, – can be recovered. However, one has to know also the exact high-momentum asymptotics of the self-energy, since the Kramers–Kronig-relations, which connect the real and imaginary parts, are integral relations. So far, we have not tried to use measured data as a starting point for constructing spectral functions as an input to our EQP-calculations. Also, for the presumed description of the whole variety of the investigated quantum channels, the generalization of our framework is needed in such a manner that conserved charges were being concerned.

Spectral functions can be also extracted from numerical simulation of a given theory (e.g. lattice-regularized QCD [7, 8, 9, 10, 11, 12]) or using other first-principle based non-perturbative methods, such as functional renormalization group (FRG) [13, 14, 15]. It would be interesting to compare the results of the EQP-calculations to the thermodynamical observables which are produced by lattice QCD in a fairly large temperature range. Using lattice QCD spectral functions as an input of the EQP, one could test in what extent the effective, extended quasi-particle treatment of the QCD degrees of freedom can reproduce the actual observables measured on a first-principle basis<sup>5</sup>. Such a systematic comparison is, however, yet to be done.

Keeping in mind that either in the case of FRG or that of lattice QCD the computation of the correlation functions of composite operators necessary to determine transport coefficients is notoriously difficult. Estimations based on EQP might offer a good guideline – at least in the case of scalar channels.

---

<sup>3</sup>This could happen when hadrons propagate through the QGP.

<sup>4</sup>It is worth mentioning that for such a decay which happens involving an intermediate resonant state the differential decay rate can be interpreted as the spectral function of the resonance, as in the case of the  $\rho$ -meson [5]. This function gives the probability that, after the resonant state decays, a hadronic state with a given mass is produced. Also, usually this function is referred to as *spectral function* in experimental reports, although it is only a contribution to the imaginary part of the quark-antiquark self-energy – for instance, see Section IV. of [6] for a thorough introduction to the decays of the  $\tau$ -lepton.

<sup>5</sup>Note, that for the real evaluation of such results it would be necessary to separate the pressure contribution of the different quantum channels – which is not typically done in lattice QCD analyses.

## References

- [1] M. Gyulassy, P. Lévai, I. Vitev and T. S. Biró,  
Phys. Rev. D **90**, 054025 (2014)
- [2] The ALEPH Collaboration,  
Phys. Rep. **421**, 191–284 (2005)
- [3] OPAL Collaboration,  
Eur. Phys. J. C **35**, 437–455 (2004)
- [4] NA60 Collaboration,  
Phys. Rev. Lett. **96**, 162302 (2006)
- [5] F. Giacosa, G. Pagliari,  
Phys. Rev. C **76**, 065204 (2007)
- [6] M. Davier, A. Hocker, Z. Zhang,  
Rev. Mod. Phys. **78**, 1043–1109 (2006)
- [7] Gert Aarts, Jose M. Martínez Resco,  
Nucl. Phys. B **726**, 93–108 (2005)
- [8] F. Karsch, E. Laermann, and S. Stickan,  
Phys. Rev. D **68**, 014504 (2003)
- [9] Péter Petreczky,  
J. Phys. G **30**, S431–S440 (2004)
- [10] Takashi Umeda, Kouji Nomura and Hideo Matsufuru,  
Eur. Phys. J. C **39S1**, 9–26 (2005)
- [11] S. Datta, F. Karsch, P. Petreczky, I. Wetzorke,  
Phys. Rev. D **69**, 094507 (2004)
- [12] A. Jakovac, P. Petreczky, K. Petrov, A. Velytsky,  
Phys. Rev. D **75**, 014506 (2007)
- [13] R.-A. Tripolt, L. von Smekal and J. Wambach,  
book chapter, arXiv:1605.00771
- [14] R.-A. Tripolt, L. von Smekal, J. Wambach and Nils Strodthoff,  
Nucl. Phys. A **931**, 790–795 (2014)
- [15] R.-A. Tripolt, L. von Smekal and J. Wambach,  
Phys. Rev. D **90**, 074031 (2014)
